# Supplementary material for: REVELIO: Universal Multimodal Task Load Estimation for Cross-Domain Generalization
Source: arXiv:2509.01642 source file (2026-11-10)
Supplement: Supplementary file 1 [file supplementary.tex]

\PassOptionsToPackage{dvipsnames}{xcolor}
\documentclass[twocolumn, 10pt, journal]{IEEEtran} 
\usepackage{amsmath,amsfonts}
\usepackage{algorithmic}
\usepackage{algorithm}
\usepackage{array}
\usepackage{subfig}
\usepackage{textcomp}
\usepackage{stfloats}
\usepackage{url}
\usepackage{verbatim}
\usepackage{graphicx}
\usepackage{cite}

\usepackage{babel}
\usepackage[T1]{fontenc}
\usepackage[utf8]{inputenc}

\usepackage{printlen}
\usepackage{layouts}
\usepackage{etoolbox}
\usepackage{tikz}

\usepackage[draft]{hyperref}

\usepackage{rotating}
\usepackage{multirow}

\usepackage{tabularx}
\usepackage{booktabs}

\usepackage{pifont}
\usepackage{colortbl}

\usepackage{amssymb}
\usepackage{nicematrix}

\usepackage{makecell}

\usepackage{url}

\usepackage[shortcuts,acronym]{glossaries}

\newacronym{facs}{FACS}{Facial Action Coding System}
\newacronym{xgb}{XGB}{Extreme Gradient Boosting}
\newacronym{ocean}{OCEAN}{Openness, Conscientiousness, Extraversion, Agreeableness, Neuroticism}
\newacronym{bfik}{BFI-K}{Big Five Inventory - Short (Kurzform)}
\newacronym{bmi}{BMI}{Body Mass Index}
\newacronym{ecg}{ECG}{Electrocardiography}
\newacronym{tlx}{TLX}{Task Load Index}
\newacronym{rtlx}{RTLX}{Raw Task Load Index}
\newacronym{pogqsf}{POGQ-SF}{Problematic Online Gaming Questionnaire Short Form}
\newacronym{adabase}{ADABase}{Autonomous Driving Cognitive Load Assessment Database}
\newacronym{isa}{ISA}{Instantaneous Self-Assessment}
\newacronym{emg}{EMG}{Electromyography}
\newacronym{eda}{EDA}{Electrodermal Activity}
\newacronym{eeg}{EEG}{Electroencephalography}
\newacronym{ppg}{PPG}{Photoplethysmography}
\newacronym{lstm}{LSTM}{long-short-term memory}
\newacronym{rnn}{RNN}{recurrent neural network}
\newacronym{cnn}{CNN}{convolutional neural network}

\begin{document}

\section{Supplementary Materials}
Additional methodological details, extended results, and configuration tables referenced in the main article are
provided in this supplementary material. This includes comprehensive descriptions of experimental protocols, data
processing pipelines, model hyperparameters, and further analyses that support the reproducibility and transparency
of our findings. Readers are encouraged to consult the supplementary document for in depth information beyond the
main text.

\subsection{Related Work Cognitive Load Measurements}
Empirical studies have evaluated cognitive load through various measurements chosen based on their sensitivity
to changes in cognitive demand, while also ensuring that these measurements do not cause external disturbances
during task execution or affect operator acceptance \cite{odonnellWorkloadAssesmentMethodology1986,
orruEvolutionCognitiveLoad2019}. The literature identifies four categories of cognitive load measures:
subjective measures, performance measures, behavioral measures, and physiological measures
\cite{chenMultimodalBehaviorInteraction2012}. \\
\emph{Subjective measurements} involve asking study participants to reflect on their perceptions through introspection
and to perform a self-assessment of their mental demand \cite{odonnellWorkloadAssesmentMethodology1986}. A widely used
technique in this category is the NASA-\gls{tlx} \cite{hartDevelopmentNASATLXTask1988} and its variations, such as the
Raw-\gls{tlx} \cite{georgssonNASARTLXNovel2020}. This technique utilizes a multidimensional measurement framework
based on factors like performance, mental effort, frustration, mental and physical demand, and temporal demand.
The limitations of subjective measures is, that these questionnaires are typically answered post-task, which means they
do not capture temporal variations \cite{paasInstructionalControlCognitive1994}. Additionally, the process, even for 
questionnaires like \gls{isa} \cite{jordanInstantaneousSelfassessmentWorkload1992}, of providing subjective feedback
can interrupt the task \cite{odonnellWorkloadAssesmentMethodology1986}. \\
\emph{Performance measurements} can reflect variations in cognitive load during a task, at least in experimental
settings. They are based on the assumption that performance will decline with an increase in cognitive load when the
capacity is overloaded \cite{paasInstructionalControlCognitive1994}. A common method is the dual-task paradigm, where
performance is evaluated for a secondary task executed in parallel. Human performance may vary with different levels of
cognitive resource activation \cite{odonnellWorkloadAssesmentMethodology1986}. However, these measurements can be
influenced by non-workload factors such as skill levels, and the secondary task can intrude on and affect primary task
performance. Typical performance measures are highly task-dependent. For instance, in studies measuring task performance
while observing an autonomous vehicle, reaction time to critical driving events or precision and recall of other events
\cite{oppeltADABaseMultimodalDataset2022} may be viable measures. In contrast, in gaming contexts, other metrics may be
more appropriate, such as the number of extinguished fires in an emergency firefighter game 
\cite{sevcenkoMeasuringCognitiveLoad2021}.\\
\emph{Behavioral responses} and features extracted from user activity are employed as measurements in various
applications. Recent studies have utilized eye-tracker-based metrics, such as fixation frequency and duration, or head
and hand movements while playing video games \cite{linEvaluatingUsabilityBased2006}. Similarly, activation and action
units extracted from facial expressions have been used in driver monitoring systems \cite{yuceActionUnitsTheir2017}. It
is important to note that behavioral measures can be consciously concealed or falsified by subjects due to trained
behaviors or may vary according to individual character or cultural background \cite{ekmanDarwinDeceptionFacial2003}.
One significant advantage of behavioral measures is that they can be recorded with minimal intrusion, allowing for
continuous monitoring while the  task is being performed.\\
This property is applicable to most \emph{physiological measurements} as well, that operate on the premise
that cognitive load corresponds to alterations in physiological processes. Such signals are frequently captured using
non-invasive sensors. For instance, the electrical activity of the heart is monitored through \gls{ecg},
activation of certain muscles related to cognitive load via \gls{emg}, and the activity of palm sweat glands
using \gls{eda}. Additionally, mechanical heart activity is assessed with \gls{ppg}, and brain activity is recorded
through \gls{eeg}. Pupil dilation, can be observed through video or specialized eye-tracker hardware 
\cite{oppeltADABaseMultimodalDataset2022}.\\
The advantage of these measurements is their applicability in laboratory experiments without disrupting most tasks
\cite{longoHumanMentalWorkload2022}. However, some extracted features may be influenced by factors other than mental 
workload \cite{cainReviewMentalWorkload2007}. Moreover, changes in biosignals occur on varying timescales. For instance, 
alterations in evoked potentials via \gls{eeg} can occur in sub-second windows, skin responses within seconds, heart
rate variability changes in the range from 30 seconds to 10 minutes, and electrogastrography typically requires window
sizes of $20$ minutes or more \cite{oppeltADABaseMultimodalDataset2022, phamHeartRateVariability2021}.\\
None of the mentioned signals are optimal, as they suffer from limitations in predictive performance, robustness, and
reliability due to the influence of external factors, with varying sensitivity across different individuals and tasks,
compounded by noise and failure from unimodal measurements, leading to the common practice of fusing and combining these
signals for assessment \cite{chenMultimodalBehaviorInteraction2012,debieMultimodalFusionObjective2021}.
\subsection{Acquisition Protocol}
Figure~\ref{app:study-protocol} presents the experimental flow chart, detailing the sequence and structure of all
study tasks. Each participant completed three main experiments $n$-back, Hogwarts Legacy, and Overcooked! 2
administered in randomized order. The protocol incorporated structured introduction phases for health assessment,
sensor setup, and eye tracker calibration, followed by baseline or training periods to ensure participant
familiarity with each task. After every major task segment, participants completed the NASA-\gls{tlx} questionnaire to
assess subjective workload. Regularly scheduled breaks, including computer guided meditation or relaxation, were
provided between sessions to mitigate fatigue and maintain baseline physiological states. Additional questionnaires
were administered during breaks and at the end of the session for comprehensive data collection. The flow chart also
indicates opportunities for task repetition and variable time intervals, ensuring that all participants could fully
understand and engage with each experiment.
\begin{figure*}
  \centering
  \noindent
  \include{tikz/study-protocol}%
  \caption{Flowchart illustrating the randomized experimentation plan across three tasks with potential repetitions,
  breaks, and debriefing phases. The experimentation plan was executed in a randomized order across all three tasks.
  %Initially, participants were assessed for health-related concerns (e.g., cardiovascular diseases, epilepsy) and
  %connected to the measurement system. Signal quality was continuously monitored and optimized before commencing the
  % first experiment.
  Breaks, meditation sessions, and the debriefing protocol were included. Meditation was computer-guided with
  controlled breathing. Dashed lines indicate variable time intervals for phases allowing participants to pause the 
  training flight, cooking sessions, or repeat $n$-back tasks to ensure adequate understanding.}
  \label{app:study-protocol}
  \vspace{-0.15cm}
\end{figure*}

\subsection{Acquisition Setup}
Figure~\ref{app:system-overview} illustrates the system architecture used for multimodal data collection. The setup
integrates a video system, Biopac physiological recording system, and game system, all synchronized via analog triggers
managed by the Biopac unit. For example, video frame acquisition is initiated by Biopac output triggers, while the
game system communicates task phase information through trigger signals. Participants are simultaneously monitored
using a camera, the Biopac system, and an eye tracker. This architecture ensures high-precision temporal alignment
across all data streams and prevents time drift between systems, thereby enabling accurate multimodal task load
detection.
\begin{figure}
  \centering
  \include{tikz/system-layout}
  \caption{System components used during data collection and their communication interfaces.}
\label{app:system-overview}
  \vspace{-0.15cm}
\end{figure}
\subsection{Demographics and Personalities}
\begin{figure}[htb!]
  \centering
  \subfloat[\centering \gls{bmi}]{\includegraphics[width=0.5\linewidth]{%
  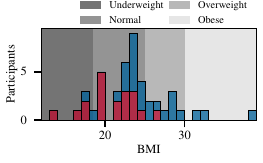}} \hfill%
  \subfloat[\centering Age Distribution]{\includegraphics[width=0.5\linewidth]{%
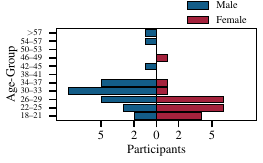}} %
  \caption{Participant demographic distribution for weight in \gls{bmi} and age.}
\label{fig:demographics}
\end{figure}
\begin{figure}[htb!]
  \centering
  \subfloat[Game Experience Questionnaire Core\label{sfig:core-game-experience-questionnaire}]{
    \includegraphics[width=1.\linewidth]{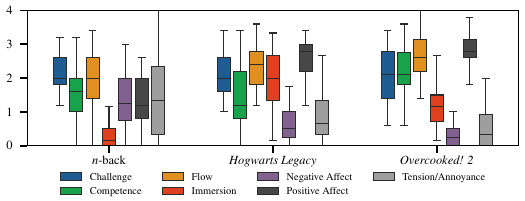}} \hfill%
  \subfloat[Post Game Experience Questionnaire\label{sfig:post-game-experience-questionnaire}]{\includegraphics[width=1.\linewidth]{%
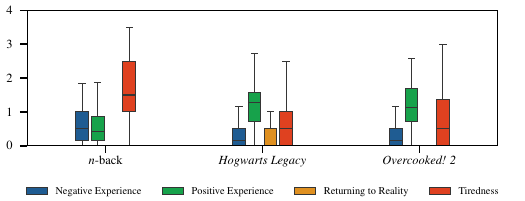}} \hfill%
  \subfloat[Intrinsic Motivation Inventory]{\includegraphics[width=1.\linewidth]{%
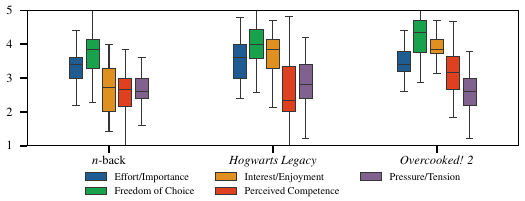}} %
  \caption{Game Experience and Intrinsic Motivation Inventory.}
\label{fig:game-experience-questionnaire}
\end{figure}
In addition to the demographic information presented in the main article, supplementary data include participants’
weight and height, with the resulting \gls{bmi} distribution shown in Fig.~\ref{fig:demographics}. We also report
participants’ task-related experiences using the Game Experience Questionnaire, with Core and Post scores visualized
in Fig.\ref{sfig:core-game-experience-questionnaire} and Fig.~\ref{sfig:post-game-experience-questionnaire},
respectively. Notably, negative affect and low immersion were most pronounced during the $n$-back task, while
both \emph{Overcooked! 2} and \emph{Hogwarts Legacy} elicited predominantly positive affect. This trend is further
supported by the Intrinsic Motivation Inventory, which revealed lower Interest and Enjoyment during $n$-back compared
to the gaming tasks. These findings suggest motivational and affective differences between cognitive testing and
gaming, highlighting an area for future investigation
\cite{jsselsteijnGameExperienceQuestionnaire2013,plantIntrinsicMotivationEffects1985}.
\subsection{Subjective}
To better understand and account for potential biases in subjective ratings, we additionally administered
the (\gls{bfik}) \cite{rammstedtKurzversionBigFive2005} to assess personality traits (\gls{ocean}). This approach
enables us to report the impact of individual personality and experience on self-reported cognitive load, thereby
improving the interpretability and validity of subjective feedback in our dataset.
To further analyze subjective questionnaire measures and especially the quality of our label annotation we collected 
personality traits. The mean \gls{ocean} personality traits are shown in Fig.~\ref{sfig:ocean_mean}, indicating that
the \gls{ocean} score distribution of our population exhibits moderate levels across all dimensions, with slightly
lower neuroticism and higher openness. As suggested by the literature \cite{rammstedtKurzversionBigFive2005}, different
personality traits may be associated with varying subjective self-assessment scores in questionnaires such as the
NASA-\gls{tlx} \cite{gjoreskiDatasetsCognitiveLoad2020}. We present the five subjects with the highest and lowest
neuroticism in Fig.~\ref{sfig:top-5-neuroticism} and the subjects with the lowest and highest level of agreeableness in
Fig.~\ref{sfig:top-5-agreeableness}. These personality traits both illustrate the distribution of characteristics
within our participant demographics and enable further analysis of character based effects on subjective assessments
(see supplementary material).
\begin{figure}[!htb]
  \centering
  \subfloat[\centering \ac{ocean} scores for all recorded subjects.\label{sfig:ocean_mean}]{%
\includegraphics[width=0.33\linewidth]{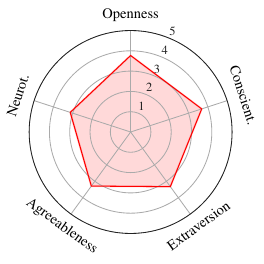}}%
  \subfloat[\centering Distribution of subjects with low and high neuroticism.\label{sfig:top-5-neuroticism}]{%
\includegraphics[width=0.33\linewidth]{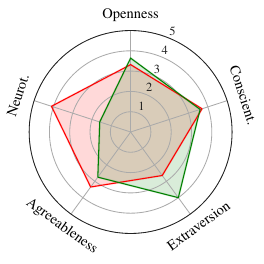}}%
  \subfloat[\centering Distributions of subjects with low and high agreeableness \label{sfig:top-5-agreeableness}]{%
\includegraphics[width=0.33\linewidth]{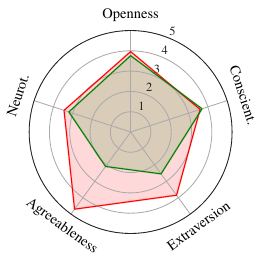}}%
  \caption{\ac{ocean} personality traits distributions of the study participants and selected subgroups.}
\label{fig:ocean_traits}
  \vspace{-0.15cm}
\end{figure}
To facilitate interpretation of our results, we include visualizations of the performance metrics originally reported
by the authors of the \gls{adabase} publication. These reference data pertain to participants who completed the 
questionnaire following the single and dual task $n$-back tests, as well as the driving test. Notably, the performance
outcomes for the single task $n$-back test are consistent with those observed in our own $n$-back experiment. These
comparative results are presented in Figure~\ref{fig:nasa-rtlx-adabase}.
We calculated the correlation between the change in \gls{rtlx} questionnaire scores from the lowest to the highest
$n$-back level and the \gls{ocean} personality traits. The analysis revealed no significant correlation ($R^2 < 0.01$),
indicating that increases in self-reported cognitive load levels is not associated with individual personality traits
in our sample population.
\begin{figure}
  \centering
  \subfloat[\centering $n$-back single]{\includegraphics[width=0.33\linewidth]{%
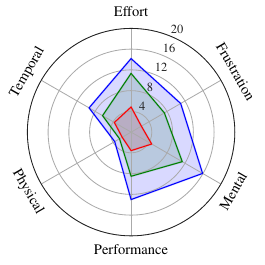}}%
  \subfloat[\centering $n$-back dual]{\includegraphics[width=0.33\linewidth]{%
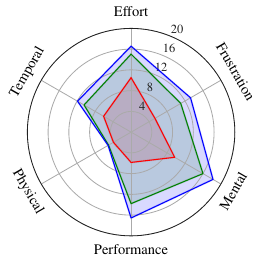}}%
  \subfloat[\centering \gls{adabase} driving]{\includegraphics[width=0.33\linewidth]{%
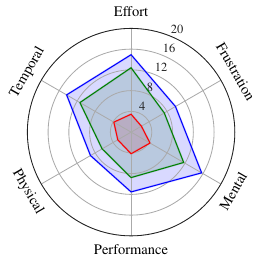}}%
  \caption{Task load indices for each dimension with increasing levels of task load (red: level 1, green level 2, blue
level 3). As supplementary illustration of our conducted experiments we evaluated the self-reported measurements from
\ac{adabase} data, showcasing single-task $n$-back with visual stimuli, dual-task $n$-back incorporating both visual
and auditory stimuli and \ac{adabase} driving.}
\label{fig:nasa-rtlx-adabase}
\end{figure}
\begin{figure*}[htb!]
  \centering
  \includegraphics{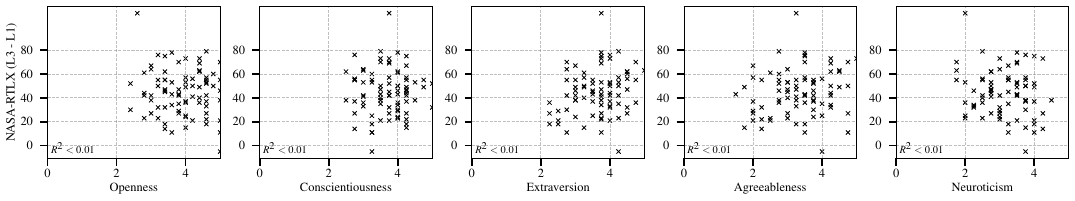}
  \caption{Correlation between \gls{ocean} triats and difference between \gls{rtlx} during maximum and minium level 
  $n$-back level. No correlation between personality traits and self-subjective rating visible.}
  \label{app:nasa-rtlx-ocean}
\end{figure*}
Consistent with the approach of \cite{oppeltADABaseMultimodalDataset2022}, we report the raw task load values in the
main text, as recommended by \cite{georgssonNASARTLXNovel2020}. For completeness and to facilitate comparison with
related studies employing weighted task load measures, we provide the corresponding weighted task load results in
Figure~\ref{app:nasa-tlx} in the supplementary materials.
\begin{figure}
  \centering
  \includegraphics{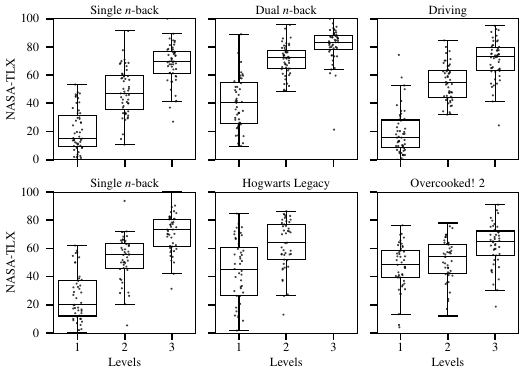}
  \caption{Weighted NASA-\ac{tlx} scores in same order and format presented as in Fig. \ref{app:nasa-tlx}.}
  \label{app:nasa-tlx}
\end{figure}
Our analysis of the correlation between the Big Five personality traits: Openness, Conscientiousness, Extraversion,
Agreeableness, and Neuroticism, assessed using the \gls{bfik}, and the increase in task load from the lowest to the
highest NASA-\gls{rtlx} scores during the $n$-back test, revealed no significant associations. This suggests that
personality traits did not substantially influence participants' subjective self-ratings of task load in this context
as shown in Figure \ref{app:nasa-rtlx-ocean}. We report the increase in NASA-\gls{rtlx} from level 1 to level 3 during
the $n$-back experiment.
\section{Reproducibility: Network Architectures}
We report network configurations with a focus on reproducibility. Model sizes reflect typical choices in affective
computing rather than optimization for computational efficiency, training time, or inference time. We also include a
large configuration for future experiments; on our baselines, moving from base to large did not improve performance.
Our objective is not to compare architectures but to demonstrate that our conclusions are dominated by the domain, not
the particular network configuration. Accordingly, we include three representative families: attention-based
transformers, convolution-based ConvNeXt and 1D ResNets, and recurrent \gls{lstm}/x\gls{lstm}models. 
\begin{table}[!htb]
  \renewcommand{\arraystretch}{1.3}
  \caption{Dimensions of the input convolution configurations.}
  \label{tab:input-dimensions}
  \begin{tabularx}{\columnwidth}{X|ccc}
  \hline
      \toprule
      Size         & Kernels    & Strides   & Channels     \\ \midrule
      \emph{tiny}  & 7, 7, 7   & 3, 3, 3   & 16, 32, 32   \\
      \emph{small} & 7, 7, 7   & 3, 3, 2   & 32, 64, 64   \\
      \emph{base}  & 7, 7, 7   & 3, 2, 2   & 64, 128, 128 \\
      \emph{large} & 7, 7, 7   & 2, 2, 2   & 128, 256, 256\\
      \bottomrule
  \end{tabularx}
\end{table}
\begin{table}[!htb]
  \renewcommand{\arraystretch}{1.3}
  \caption{Dimensions of the LSTM configurations.}
  \label{tab:lstm-dimensions}
  \begin{tabularx}{\columnwidth}{X|cc}
  \hline
      \toprule
      Size         & Hidden Size & Layers \\ \midrule
      \emph{tiny}  & 64         & 2      \\
      \emph{small} & 128        & 4      \\
      \emph{base}  & 256        & 8      \\
      \emph{large} & 512        & 16     \\
      \bottomrule
  \end{tabularx}
\end{table}
We use the architectures described in the main text: \gls{lstm}–based recurrent neural networks
(historically employed for affective time-series processing \cite{gjoreskiMachineLearningEndtoEnd2020}) shown in
\ref{tab:lstm-dimensions}; 1D ResNet-18, ResNet-34, and ResNet-50 encoders, previously used in affective computing
\cite{jinHumanCentricCognitiveState2025,wangTimeSeriesClassification2017}; a time-series transformer
\cite{jinHumanCentricCognitiveState2025,wenTransformersTimeSeries2023}; ConvNeXt adapted to 1D
\cite{liuConvNet2020s2022}; and x\gls{lstm}\cite{beckXLSTMExtendedLong2024}.
For both \gls{rnn} (\gls{lstm}: \footnote{LSTM: \url{https://github.com/pytorch/pytorch/blob/v2.6.0/torch/nn/modules/rnn.py}}
and x\gls{lstm} \footnote{x\gls{lstm}: \url{https://github.com/NX-AI/xlstm/releases/tag/v2.0.3}}) and transformer models, we employ
a 1D convolutional input front end configured as in Table~\ref{tab:input-dimensions}. The final sequence representation
is aggregated by mean over time and passed through a linear projection for classification. Transformer encoders
\footnote{Transformer: \url{https://github.com/pytorch/pytorch/blob/v2.6.0/torch/nn/modules/transformer.py}} use the
same input front end, followed by depth,
width, and attention settings as in Table~\ref{tab:transformer-dimensions}. For x\gls{lstm}-based networks, established
hyperparameters are limited; we therefore defined custom configurations in which the \emph{tiny}, \emph{small},
\emph{base}, and \emph{large} variants use 2, 4, 8, and 16 m\gls{lstm} and s\gls{lstm} heads, respectively
(Table~\ref{tab:xlstm-dimensions}). The \gls{cnn} backbones (1D ResNet 
\footnote{ResNet \url{https://github.com/pytorch/vision/blob/release/2.0/torchvision/models/resnet.py}} and ConvNeXt
\footnote{ConvNeXt \url{https://github.com/facebookresearch/ConvNeXt}}) do not use this shared front-end.
For \gls{cnn}-based models, we implement 1D versions of ResNet-18, ResNet-34, and ResNet-50
\cite{jinHumanCentricCognitiveState2025,wangTimeSeriesClassification2017}. For ConvNeXt, we use the \emph{tiny},
\emph{small}, \emph{base}, and \emph{large} variants \cite{liuConvNet2020s2022}, adapting all 2D convolutions to 1D
with per-stage dimensions in Table~\ref{tab:convnext-dimensions}.
All model hyperparameters (layers, filters, kernel sizes, dropout rates, and activations) follow established
literature and original codebases. These implementation details are provided primarily to support reproducibility and
to enable future studies to build on our configurations; they are not intended to represent optimally tuned,
cross-architecture–comparable settings.
\begin{table}[!htb]
  \renewcommand{\arraystretch}{1.3}
  \caption{Dimensions of the Transformer configurations.}
  \label{tab:transformer-dimensions}
  \begin{tabularx}{\columnwidth}{X|ccccc}
  \hline
      \toprule
      Size         & Layers & Dimension & Heads & Feed Forward & Dropout \\ \midrule
      \emph{tiny}  & 6     & 32       & 8     & 1024    & 0.05    \\
      \emph{small} & 8     & 64       & 8     & 2048    & 0.10    \\
      \emph{base}  & 12    & 128      & 16    & 3072    & 0.15    \\
      \emph{large} & 24    & 256      & 32    & 4096    & 0.20    \\
      \bottomrule
  \end{tabularx}
\end{table}
\begin{table}[!htb]
  \renewcommand{\arraystretch}{1.3}
  \caption{Dimensions of the xLSTM configurations.}
  \label{tab:xlstm-dimensions}
  \begin{tabularx}{\columnwidth}{X|cc}
  \hline
      \toprule
      Size         & MLSTM Heads & SLSTM Heads \\ \midrule
      \emph{tiny}  & 2          & 2           \\
      \emph{small} & 4          & 4           \\
      \emph{base}  & 8          & 8           \\
      \emph{large} & 16         & 16          \\
      \bottomrule
  \end{tabularx}
\end{table}
\begin{table}[!htb]
  \renewcommand{\arraystretch}{1.3}
  \caption{Dimensions of the ConvNeXt configurations per stage.}
  \label{tab:convnext-dimensions}
  \begin{tabularx}{\columnwidth}{X|l|ccc}
  \hline
      \toprule
      Size & Stage & in & out & layers \\ \midrule
      \multirow{4}{*}{\emph{tiny}} 
        & 1 & 96  & 192  & 3  \\
        & 2 & 192 & 384  & 3  \\
        & 3 & 384 & 768  & 9  \\
        & 4 & 768 & -    & 3  \\ \midrule
      \multirow{4}{*}{\emph{small}}
        & 1 & 96  & 192  & 3  \\
        & 2 & 192 & 384  & 3  \\
        & 3 & 384 & 768  & 27 \\
        & 4 & 768 & -    & 3  \\ \midrule
      \multirow{4}{*}{\emph{base}}
        & 1 & 128 & 256  & 3  \\
        & 2 & 256 & 512  & 3  \\
        & 3 & 512 & 1024 & 27 \\
        & 4 & 1024& -    & 3  \\ \midrule
      \multirow{4}{*}{\emph{large}}
        & 1 & 192 & 384  & 3  \\
        & 2 & 384 & 768  & 3  \\
        & 3 & 768 & 1536 & 27 \\
        & 4 & 1536& -    & 3  \\
      \bottomrule
  \end{tabularx}
\end{table}
\subsection{Computational Complexity}
All model training was conducted on a Nvidia RTX 4090 GPU. To ensure robust model evaluation, we employed five-fold
cross-validation throughout all experiments.
For this publication, we deliberately refrained from extensive hyperparameter optimization or micro-optimization, as
our primary objective was to provide a comprehensive overview rather than to maximize individual model performance, but
create this subject-wise splitting strategy for future work to build upon.
In the case of our baseline models, we considered five outer test folds, five distinct dataset configurations, three
different model sizes, and three architectural types, resulting in a broad exploration of model variants. The
total runtime was approximately seven days.
For experiments involving our multimodal setup, we evaluated three architectural variants across five datasets and
five outer folds, encompassing a total of 21 unique model-dataset combinations. The total runtime was approximately 25
days.
All models were trained using the Adam optimizer, with a weight decay of 0.000001 and a learning rate of 0.00001. We
employed a scheduler to reduce the learning rate on plateau, using a reduction factor of 0.5 and a patience parameter
of 16 epochs. Early stopping was implemented with a patience of 32 epochs, and all models were trained for a maximum
of 128 epochs.
\subsection{Splitting Strategy}
To prevent data leakage, we implement a $k$-fold subject-wise (grouped) stratified (experiments) cross-validation
strategy, ensuring that records from subjects who participated twice are assigned to the same fold. The dataset is
divided into $k$ equally sized groups: $k-2$ folds are used for training, one for validation, and one for testing.
The inner splits are utilized for training and validation, including procedures such as early stopping, while the
outer folds assess model performance on unseen data and subjects. This approach enables robust evaluation by reporting
the mean and standard deviation of performance metrics across multiple folds, thus preventing data leakage.

\bibliographystyle{IEEEtran}
\bibliography{bibliography}

\end{document}
